# Supplementary material for: Generative Novel View Synthesis with 3D-Aware Diffusion Models
Source: arXiv:2304.02602 source file (2023-04-05)
Supplement: Supplementary file 1 [file visual_results.tex]

\section{Additional visual results}
\label{sec:supp_visual_results}
\kn{this section should have "demo" results without comparisons. qualitative results with comparisons should go to Sec.1}
\subsection{ShapeNet}

\begin{figure*}[h]
    \centering
    \includegraphics[width=\textwidth]{example-img-a}
    \caption{Caption}
    \label{fig:my_label}
\end{figure*}

\subsection{Matterport 3D}

\begin{figure*}[h]
    \centering
    \includegraphics[width=\textwidth]{example-image-b}
    \caption{Caption}
    \label{fig:my_label}
\end{figure*}

% \twocolumn[{%
% \renewcommand\twocolumn[1][]{#1}%
% \maketitle
% \begin{center}
%     \vspace{-0.5cm}
%     \centering
%     \captionsetup{type=figure}
%     \includegraphics[width=\textwidth]{images/teaser_mp3d.pdf}
%     \vspace{-0.25in}
%     \captionof{figure}{\kn{is there some kind of "frames" that indicate how far apart these images are?}}
%     \label{fig:teaser}
% \end{center}%
% }]
